# Supplementary material for: On Learning Rates and Schr\"odinger Operators
Source: arXiv:2004.06977 source file (2020-04-15)
Supplement: Supplementary file 1 [file sec_prob.tex]

\section{Proof of Section~\ref{sec: prob_single}}
\label{sec: proof_prob_single}

%%%%%%%%%%%%%%%%%%%%%%%%%%%%%%%%%%%%%%%%%%%%%%%%%%%
\subsection{Proof of Lemma~\ref{lem: gronwall-continuity}}
\label{subsec: proof-gron-cont}
Recall the~\textit{High-Resolution} SDE~\eqref{eqn: sgd_high_resolution} and standard gradient flow~\eqref{eqn: sgd_low_resolution},
with the same initial $X(0) = x_{0}$, we have
\[
X_{s}(t) - X_{0}(t) = \int_{0}^{t} \left[ \nabla f(X_{s}(u)) - \nabla f(X_{0}(u)) \right] \dd u + \sqrt{s} W(t).
\]
Since $f \in C_{L}^{\infty}(\mathbb{R}^{d})$, we can obtain further
\[
\left\| X_{s}(t) - X_{0}(t) \right\| \leq L \int_{0}^{t} \left\| X_{s}(u) - X_{0}(u) \right\| \dd u +  \sqrt{s} \|W(t)\|.
\]
Taking the supremum on $[0, T]$, we have 
\begin{align*}
\sup_{0\leq t \leq T} \left\| X_{s}(t) - X_{0}(t) \right\| & \leq L \sup_{0\leq t \leq T} \int_{0}^{t} \left\| X_{s}(t) - X_{0}(t) \right\| \dd u +  \sqrt{s} \sup_{0\leq t \leq T} \|W(t)\| \\
                                                                                & \leq L  \int_{0}^{T} \sup_{0\leq u \leq t} \left\| X_{s}(u) - X_{0}(u) \right\| \dd u +  \sqrt{s} \sup_{0\leq t \leq T} \|W(t)\|
\end{align*}
By Gr\"{o}nwall's inequality, we can obtain
\[
\sup_{0\leq t \leq T} \left\| X_{s}(t) - X_{0}(t) \right\| \leq  \sqrt{s} \sup_{0\leq t \leq T} \|W(t)\| e^{LT}.
\]

%%%%%%%%%%%%%%%%%%%%%%%%%%%%%%%%%%%%%%%%%%%%%%%%%%%
\subsection{Proof of Lemma~\ref{lem: d-gaussian}}
\label{subsec: proof-d-gaussian}

For each component of $X$, $X_{i} \sim \mathcal{N}(0,1)$ ($i = 1, \ldots, d$),  we know $\|X\|^{2} \sim \chi^{2}(d)$.
Hence, for any $x>0$, we can obtain
\[
\mathbf{Pr}(\|X\| \geq x) = \mathbf{Pr}(\|X\|^{2} \geq x^{2}) = \frac{ \Gamma\left( \frac{d}{2}, \frac{x^{2}}{2}\right) }{\Gamma\left( \frac{d}{2} \right)},
\]
where $\Gamma(\cdot, \cdot)$ is the upper incomplete gamma function as
\[
\Gamma\left( \frac{d}{2}, \frac{x^{2}}{2} \right) = \int^{\infty}_{\frac{x^{2}}{2}} t^{\frac{d}{2} - 1} e^{-t} \dd t
\] 
and $\Gamma(\cdot)$ is the complete gamma function as
\[
\Gamma\left( \frac{d}{2} \right) = \int^{\infty}_{0} t^{\frac{d}{2} - 1} e^{-t} \dd t.
\] 
By the asymptotic property of the upper incomplete gamma function, we know that there exists $x_{0} > 0$ and some constant $C>0$ such that for any $x > x_{0}$
\[
\Gamma\left( \frac{d}{2}, \frac{x^{2}}{2} \right) \leq \frac{2  x^{d - 2} 2^{1 - \frac{d}{2}}e^{- \frac{x^{2}}{2}}}{\Gamma\left( \frac{d}{2}\right)} = \frac{4 x^{d - 2} e^{-\frac{x^{2}}{2}}}{2^{\frac{d}{2}} \Gamma\left( \frac{d}{2}\right)}
\]

%%%%%%%%%%%%%%%%%%%%%%%%%%%%%%%%%%%%%%%%%%%%%%%%%%%%%
%%%%%%%%%%%%%%%%%%%%%%%%%%%%%%%%%%%%%%%%%%%%%%%%%%%
\subsection{Proof of Lemma~\ref{lem: gronwall-discrete}}
\label{subsec: proof-gron-disc}

Recall the SGD~\eqref{eqn: sgd_constant} and GD~\eqref{eqn: GD_constant_step}, with the same initial, we have
\[
x_{s, k} - x_{0, k} =  s \left( \nabla f(x_{s, k-1}) - \nabla f(x_{0, k-1}) \right) + s \xi.
\]
Since $f \in C_{L}^{\infty}(\mathbb{R}^{d})$, we can obtain further
\[
\| x_{s, k} - x_{0, k} \| \leq L \| x_{s, k-1} - x_{0, k-1} \| + s \|\xi_{k}\|.
\]
Hence, with the above recursion relation, we have
\[
\| x_{s, k} - x_{0, k} \| \leq  s (1 + Ls)^{\frac{T}{s}} \sup_{0\leq k \leq T/s}\|\xi_{k}\| \leq s \sup_{0\leq k \leq T/s}\|\xi_{k}\| e^{LT}.
\]
